# Supplementary material for: CadVLM: Bridging Language and Vision in the Generation of Parametric CAD Sketches
Source: arXiv:2409.17457 source file (2024-09-26)

Original

Input

Sampling output

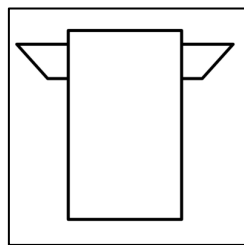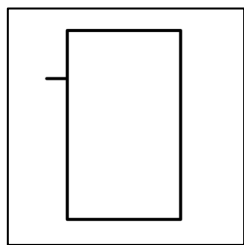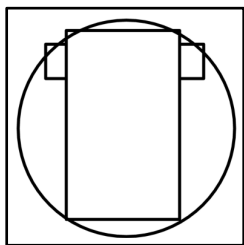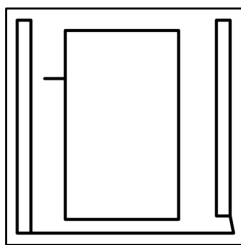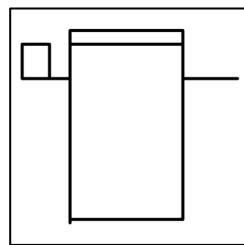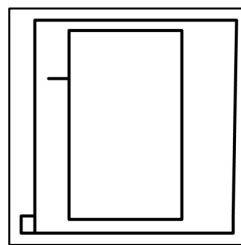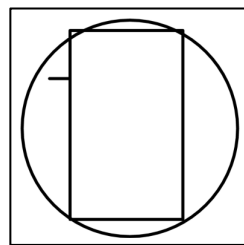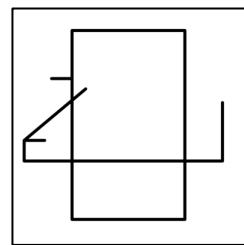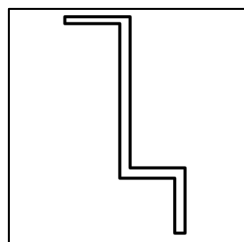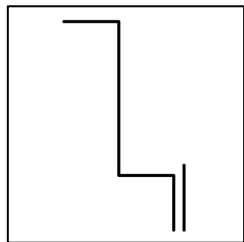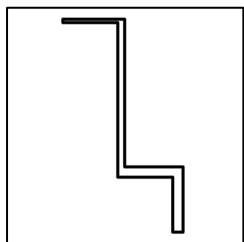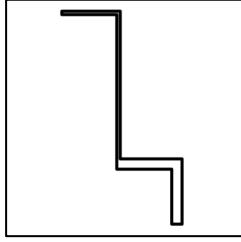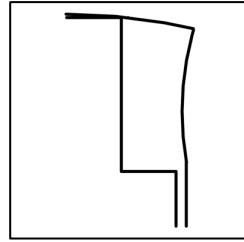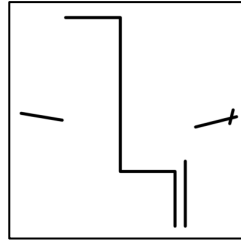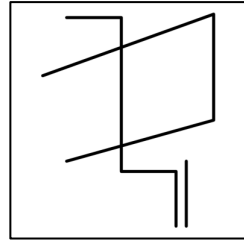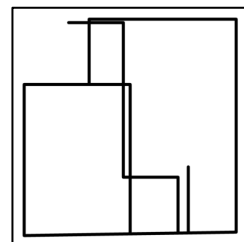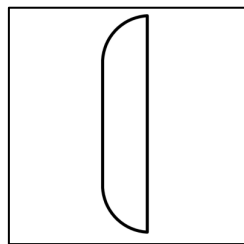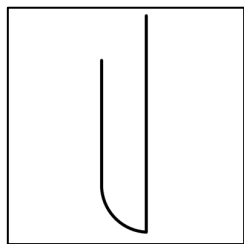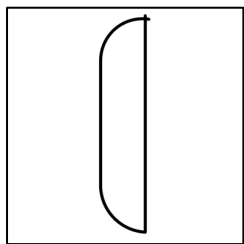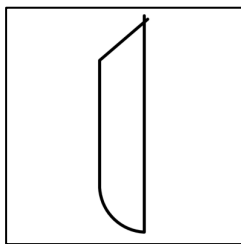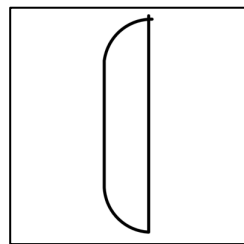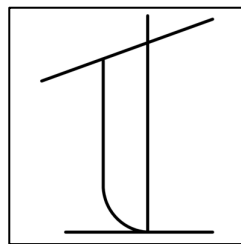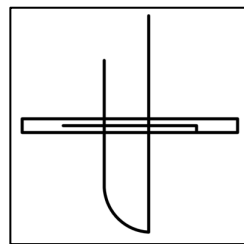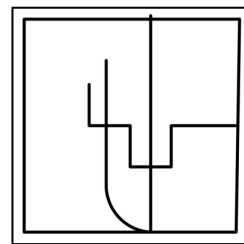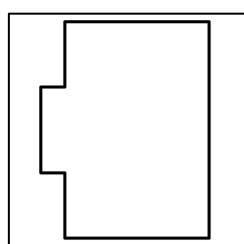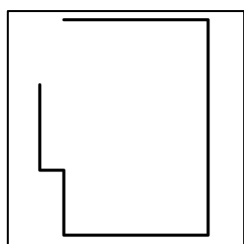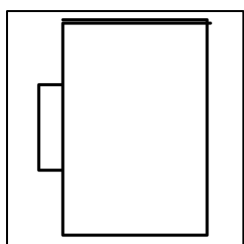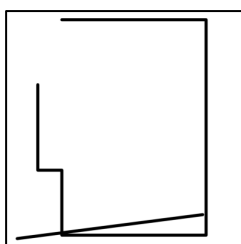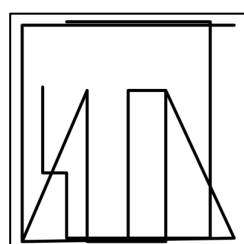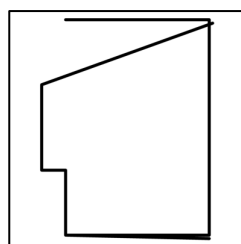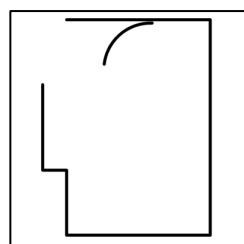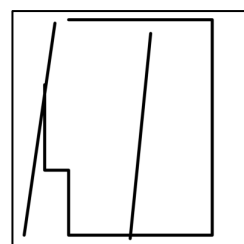

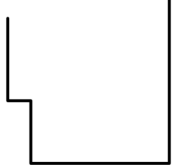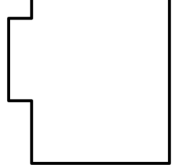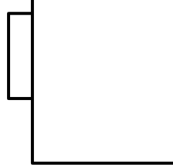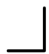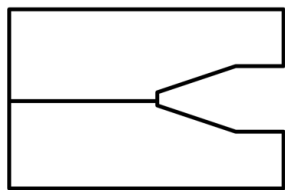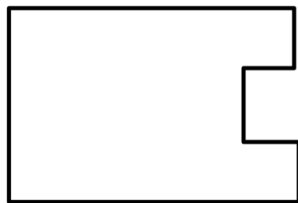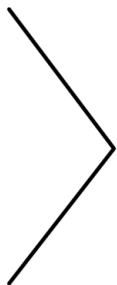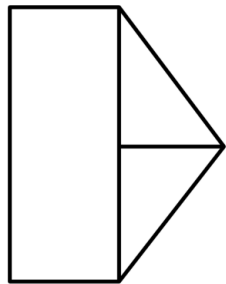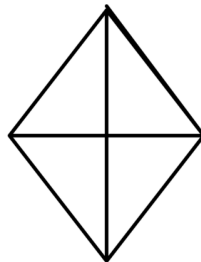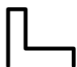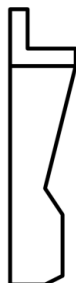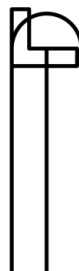

Supplement: Supplementary file 1 [file supp_multisampling.pdf]
